# Supplementary material for: The evaporation of charged black holes
Source: arXiv:2411.03447 source file (2024-11-05)
Supplement: Supplementary file 1 [file oldappendix.tex]

\section{Accounting for metric fluctuations in the near-horizon region}

In this section we will closely follow the strategy of \cite{} to find various production rates for particles affected by the near-horizon quantum fluctuations. The general strategy will be to write the particle occupation number using a double integral over the boundary 

\subsection{Conventions for the metric}
The standard Poincar\'e metric is given by 
\be 
ds^2 = \frac{dz^2 + d\tau^2}{z^2} = \frac{dw d\bar w}{(w+\bar w)^2}
\ee
where $w = z+i \tau$ and $\bar w = z-i \tau$. When using Dirichlet boundary conditions, the boundary of $AdS_2$ is fixed such that $g_{uu} = 1/\epsilon^2$ where $\int du \sqrt{g_{uu}} = \beta/\e$, where $u$ is the proper time of some observer leaving on the boundary which will be detecting the particles which are outgoing from the bulk. This implies that in terms of the boundary time $u$
\be 
\frac{(z')^2 + (\tau')^2}{z^2} = \frac{1}{\e^2}
\ee
from which one finds that $z = \epsilon \tau' + O(\epsilon^2)$. In terms of $w$ and $\bar w$ this means that $w+\bar w  = -i\epsilon(w'-\bar w') + O(\epsilon^2)$, which implies that $w = -\bar w - 2i\epsilon \bar w' + O(\epsilon^2)$. We will now write $w = \tau(v)$ and $\bar w = -\tau(\bar v)$ where we analytically continue the function $\tau(v)$ to the complex plane.\footnote{A relation that will prove useful is \be 
z = \frac{\tau(v)-\tau(\bar v)}2\,, \qquad \tau  = -i\frac{\tau(v)+\tau(\bar v)}2\,.
\ee
} 
The metric then becomes
\be 
\label{eq:bilocal-metric}
ds^2=-\frac{\tau'(\bar v) \tau'(v)}{(\tau(\bar v)-\tau(v))^2} d\bar v dv 
\ee
where the boundary is placed at $\tau(v(u))-\tau(\bar v(u)) = -2i \epsilon \tau'(\bar v(u)) \bar v'(u) +  O(\epsilon^2)$ which is solved by $\bar v(u) = v(u) +2i \epsilon v'(u) + O(\epsilon^2)$. We will be interested in the case for which $v(u) = u$ on the boundary, for which $\bar v(u) = u + 2i \epsilon + O(\epsilon^2)$. When doing this, we will from now on label $\bar v = \bar u$. This metric is useful in defining diffeomorphism invariant operators in the bulk.

Finally, the observer that we are interested in is the Rindler observer for which we have to reparametrize $\tau(u) = \tanh\left(\frac{\pi}{\beta}f(u)\right)$ with $f(u+\beta) = f(u) + \beta$. In such a case, the metric \eqref{eq:bilocal-metric} becomes 
\be 
ds^2=-\frac{\pi^2 f'(\bar u) f'(u)}{\beta^2 \sinh\left[\frac{\pi}{\beta} f(\bar u)-f(u)\right]^2} d\bar u du 
\ee
Our observer will measure energies with respect to the time $t$, defined by $u = it+x$, $\bar u = -it+x$.

We can recover the standard ``Schwarzschild'' coordinates, which corresponds to the trivial configuration, $f(u) = u$, by taking $u = it+x$, $\bar u = -it+x$:
\be 
\label{eq:Schwarzild-metric}
ds^2=-\frac{(\pi/\beta)^2}{\sinh\left(\frac{\pi}{\beta}x\right)} (dx^2 - dt^2)
\ee
Finally to obtain the standard metric for the RN black hole one simply needs to perform a reparametrization of the coordinate $x$ in \eqref{eq:Schwarzild-metric}, without changing the time $t$.

To compare some of our results to previous Schwinger production computations \cite{}, we will also the coordinates 
\be
ds^2= e^{2x} dt^2 + dx^2
\ee
which is related to the Poincar\'e coordinates above 
\be 
x = - \log z,\, \qquad t= {\tau}\,.
\ee
where the boundary of AdS$_2$ is located at $z \to 0$ and $x \to \oo$ and the ``horizon'' is located at $z \to \oo$ and $x \to -\oo$. 

\subsection{Neutral free scalar particles}

We will be interested in coupling the theory to a scalar field whose action is given by 
\be 
I_\text{matter} = \int d^4x \sqrt{g} \left[(\partial_\mu \phi)^2 + m^2 \phi^2\right]
\ee
The equation of motion for the field $\phi$ is given by the Klein-Gordon equation 
\be
-\partial_\tau^2 \phi(z, \tau)^2 +\partial_z^2 \phi(z, \tau)- \frac{m^2}{z^2} \phi(z, \tau) = 0  \,,
\ee
in Poincar\'e coordinates, in Lorentzian signature, or
\be 
4 {\partial_u \partial_{\bar u}}\phi(u, \bar u) - 4 m^2 \frac{\tau'(u) \tau'(\bar u)}{(\tau(u)-\tau(\bar u))^2}\phi(u, \bar u) = 0\,,
\ee
in the bilocal coordinates \eqref{eq:bilocal-metric}. 
We are interested in ``in''-states given by the vacuum defined by the annihilation operators which obtained in the mode decomposition  
\be
\phi = \int d\omega\left[a^\dagger_\Poi \phi_{-\omega}^{\text{(in)}} e^{i \omega \tau} + a_\Poi \phi_{\omega}^{\text{(in)}} e^{-i \omega \tau} \right]\,, \qquad a_\Poi|0\>_\text{(in)} = 0\,,
\ee
with respect to the Poincar\'e time $\tau$ and in using a Rindler observer defined by the mode decomposition 
\be
\phi = \int d\omega\left[a^\dagger_\Rin \phi_\omega^{\text{(out)}} e^{i \omega t} + a_\Rin \phi_{-\omega}^{\text{(out)}} e^{-i \omega t} \right]\,.
\ee
We are interested in solving for $\phi_{(\omega)}^{\text{(in)}}$ on the entire AdS$_2$ space and  $\phi_{(\omega)}^{\text{(out)}}$ close to the boundary of AdS$_2$.\footnote{We will however only use the boundary two-point function measured with respect to the ``in''-state.} The solution for $\phi^{(in)}_\omega$ is well known and is given by 
\be 
\phi^{\text{(in)}}_\omega(z) = \sqrt{\frac{z}2} J_{h-\frac{1}2}(\omega z)
\ee
where $m^2 = h(h-1)$ for $m \neq 0$, and by 
\be 
\phi^{\text{(in)}}_\omega(z) = \frac{\sin(\omega z)}{\sqrt{\pi \omega}}
\ee
for $m = 0$. We can check the normalization by noting that the Klein-Gordon inner product is given by
\be 
\< \phi_1, \phi_2\> = \int_\Sigma dx \sqrt{h} (\phi_2 n^a \partial_a \phi_1 - \phi_1 n^a \partial_a \phi_2)
\ee
on some curve $\Sigma$, where $h$ is the induced metric by $g_{\mu \nu}$ on $\Sigma$ and $n^a$ is the unit normal vector to $\Sigma$ with $n^a n_a = 1$. Thus, we have that for instance
\be 
\<\phi_{\omega_1}^\text{(in)} e^{i \omega_1 t}, (\phi_{\omega_2}^\text{(in)}  e^{i \omega_2 t})^*\> = \frac{1}\pi \sqrt{\frac{\omega_2}{\omega_1}}\int_0^\infty dz \sin(\omega_1 z) \sin(\omega_2 z) e^{i t(\omega_1 - \omega_2)} = \delta(\omega_1 - \omega_2)
\ee

Close to the boundary, the two-point function measured with respect to the ``in''-vacuum is given by 
\be
\lim_{z_1, z_2\to 0}\,\<0|_\text{in} \phi(z_1, \tau_1) \phi(z_2, \tau_2) |0\>_\text{in} = \frac{1}{|\tau_1 - \tau_2|^{2h}}
\ee

In the bi-local coordinates, close to the boundary, we can expand the Klein-Gordon equation for  $\phi$ and rewrite is as, 
\be 
\frac{m^2 \phi(u, \bar u)}{(u-\bar u)^2} + \partial_u \partial_{\bar u} \phi(u, \bar u) + \underbrace{O\left((u-\bar u)^2\right)}_{O(\e^2)}= 0\,.
\ee
Thus, close to the boundary $\phi^{\text{(out)}}_\omega$ satisfies  
\be
\phi^{\text{(out)}}_\omega(x)''+ \omega^2 \phi^{\text{(out)}}_\omega(x) - \frac{m^2}{x^2} \phi^{\text{(out)}}_\omega(x) + O(x^2) = 0
\ee
which is the same as the Klein-Gordon  in Poincar\'e coordinates. Thus, the solution close to the boundary is again 
\be 
\phi^{\text{(out)}}_\omega(x) = \sqrt{\frac{x}2} J_{h-\frac{1}2}(\omega x) =_{\lim x\to 0} x^h \left(\frac{(\omega/2)^{h-\frac{1}2 }}{\Gamma\left(\frac{1}2 +h \right)}+O(x^2)\right)
\ee
which for $h>0$ vanishes as $x\to 0$. There is another solution given by 
\be
\sqrt{\frac{x}2} J_{\frac{1}2-h}(\omega x)
\ee
which diverge as $x\to 0$.\LVI{so perhaps should be thrown out since it won't be normalizable?}
The normalization of $\phi^{\text{(out)}}_\omega(x)$ is again fixed by the Klein-Gordon inner-product defined with respect to the curve of constant $t$. We now want to analytically continue the Klein-Gordon inner product along some complex contour for which the metric is Euclidean. In such a case, the orthogonaltiy properties still hold and the particle-number can be written as 
\be
\<N_\omega\> = -\int_{\bar u_1 = u_1+2i\e, {\bar u_2 = u_2+2i\e}} dt_1 dt_2 \phi^{\text{(out)}}_\omega(x_1, t_1) \phi^{\text{(out)}}_\omega(x_2, t_2)^*  :\<0|_\text{in}\partial_{t_1}\phi(x_1, t_1) \partial_{t_2}(x_1, t_1)\phi|0\>_\text{in}:
\ee
\LVI{Still confused about contours?} . This is given by 
\be 
\<N_\omega\> = \int du_1 du_2\,\, \phi^{\text{(out)}}_\omega(u_1) \phi^{\text{(out)}}_\omega(u_2)^*\,\, \frac{2h(1+2h)F'(u_1)F'(u_2)}{(F(u_1)-F(u_2))^{2h+2}}
\ee
\LVI{This formula needs some divergence curing?}

\textbf{Classical behaviour.} \,\,\, Let's first look at the classical saddle of the Schwarzian theory for which $F(u) = \tanh(\frac{\pi}{\beta} u)$. This means that  
\be 
\<N_\omega\>& = \int du_1 du_2\,\, \phi^{\text{(out)}}_\omega(u_1) \phi^{\text{(out)}}_\omega(u_2)^*\,\, \frac{2h(1+2h)}{\sinh\left(\frac{\pi}{\beta}u_{12}\right)^{2h+2}}\nn \\
&= \frac{2h(1+2h)\epsilon^{2h}(\omega/2)^{2h-1}}{\Gamma\left(\frac{1}2 +h\right)^2 } \delta(0)\int du_{12}\,\, \frac{e^{i\omega u_{12}}}{\sinh \frac{\pi u_{12}}{\beta}}\,.
\ee
We can do the integral exactly to find that 
\be
\<N_\omega\>
\ee

\subsection{Neutral free fermionic particles}

\subsection{Charged scalar particles}

We now consider the coupling the coupling to a charged scalar field, \be
I_\text{matter} = \int d^4x \sqrt{g} \left[(D_\mu \phi)^2 + m^2 \phi^2\right]
\ee
with $D_{\mu} = \partial_\mu - i q A_\mu$. We will expand the field $\phi$ as, 
\be 
\phi(t, x) = \int_0^\infty \frac{d\omega}{2\pi} \left[\tilde\phi_{-\omega}(x) e^{+i \omega t} + \tilde\phi_{\omega}(x) e^{-i \omega t}\right]
\ee
where $\tilde \phi_\omega$ obeys 
\be 
\left[e^{- x} \partial_x(e^{ x} \partial_x) + e^{-2  x} \left( \omega - {q E}e^{x} \right)^2 - m^2 \right] \tilde \phi_\omega(x) = 0\,.
\ee
which in Poincar\'e coordinates is given by 
\be 
\frac{1}{ z^2}\left[-{m^2} + \left({q E} - z\omega \right)^2 \right] \tilde \phi_\omega+ \tilde \phi_\omega'' = 0 
\ee  
We first wish to write $\tilde \phi_\omega(x)$ in such a way that it is well behaved as $x \to -\oo$. This is given by a linear combination of the two solutions
\be 
\tilde \phi_{\omega}^{\text{in, }(+)} \sim W_{\kappa, -\nu}(\zeta) \,, \qquad \tilde \phi_{\omega}^{\text{in, }(-)}  \sim W_{\kappa, -\nu}(-\zeta) \,.
\ee
where $W_{\kappa, -\nu}(\zeta)$ is the Whittaker W-function whose labels are given by 
\be 
\kappa = i {q E}\,, \qquad \nu = {i \gamma_{AdS}} = i {\sqrt{\left({qE}\right)^2 - \left(m^2+\frac{1}4\right)}}\,, \qquad \zeta = 2i {\bar{\omega}} e^{-  x} = 2i {\bar \omega z }\,, \qquad \bar \omega = \omega - {qE}\,.
\ee
To see that the Whittaker functions are well behaved as $z \to \oo$, $x \to -\oo$ and $|\zeta| \to \infty$ we use the expansion $W_{\kappa, \nu}(\zeta) =_{|\zeta|\to \infty} e^{-\zeta/2} \zeta^\nu\left[1+O(1/\zeta)\right]$. This means that as $z \to \infty$ 
\be 
\tilde \phi_{\omega}^{\text{in, }(+)}(z) \sim e^{-i {\bar \omega z} + O(\log z)}\,, \qquad \tilde \phi_{\omega}^{\text{in, }(-)}(z) \sim e^{i {\bar \omega z}+ O(\log z)}\,.
\ee
Thus, $\tilde \phi_{\omega}^{\text{in, }(+)}(\zeta)$ is the mode going into the $AdS_2$ bulk and $\tilde \phi_{\omega}^{(+)}(\zeta)$ is the mode going out from the $AdS_2$ bulk into the horizon. 

Similarly, we can impose that the field $\phi$ is well behaved close to the AdS$_2$ boundary. These are given by 
\be 
\tilde \phi^{\text{out, }(+)}_\omega(x) \sim M_{\kappa, -\nu}(\zeta)\,,\qquad \phi^{\text{out, }(-)}_{\omega}(x) \sim  M_{\kappa, \nu}(\zeta)\,.
\ee
As $z \to 0$, $x \to \oo$ and $|\zeta| \to 0$ we have that $M_{\kappa, \nu}(\zeta) =_{|\zeta|\to \infty} \zeta^{\nu + \frac{1}2}\left[1+O(1/\zeta)\right]$. Thus, we have that
\be
\tilde \phi^{\text{out, }(+)}_\omega(x) \sim e^{\left(\nu-\frac{1}2  \right) x}\,, \qquad \tilde \phi^{\text{out, }(-)}_\omega(x) \sim e^{\left(-\nu-\frac{1}2  \right) x}
\ee
where, since $\nu \in i \mathbb R^+$, we can interpret $\tilde \phi^{\text{out, }(+)}_\omega(x)$ as the outgoing mode for a particle leaving a near-horizon region and $\tilde \phi^{\text{out, }(-)}_\omega(x)$ as the ingoing mode of a particle entering the near-horizon region. 

We wish to impose absorbing boundary conditions at the boundary of $AdS_2$ and thus solely keep the $\tilde \phi^{\text{out, }(+)}_\omega(x)$ mode. This implies that at the boundary  the mode decomposition takes the form 
\be
\phi = \int_0^\infty d\omega \left[a_\omega^\dagger \phi^{\text{out, }(+)}_{-\omega}(x) e^{i \omega t}+b_\omega  \phi^{\text{out, }(+)}_{\omega}(x) e^{-i \omega t} \right]
\ee
where 
\be 
\phi^{\text{out, }(+)}_{\omega}(x) = \left(\frac{1}{2i\bar \omega}\right)^{1/2} \left(\frac{1}{2\gamma_{AdS}}\right)^{1/2} M_{\kappa, -\nu}(\zeta)
\ee
where the normalization is given such that 
\be
\label{eq:normalization-condition}
-i\int dx \sqrt{g_{xx}} \text{Wr}[\phi^{\text{out, }(+)}_{\omega_1}(x)^*, \phi^{\text{out, }(+)}_{\omega_2}(x)] = \delta(\omega_1 - \omega_2)\,,
\ee
where \text{Wr} is the Wronskian. This is satisfied since the Whittaker functions have the property that $e^{- x}\,\text{Wr}[\phi^{\text{out, }(+)}_{\omega}(x)^*, \phi^{\text{out, }(+)}_{\omega}(x)] =i$, where we note that $\phi^{\text{out, }(+)}_{\omega}(x)^* =\phi^{\text{out, }(-)}_{\omega}(x)$.\footnote{Note that however $\phi^{\text{out, }(+)}_{\omega}(x)^* \neq \phi^{\text{out, }(+)}_{-\omega}(x)$ which is what would happen in the absence of an electric field.}

We can now write the quantization of the field in terms of creation and annihilation operators that act on the in-vacuum. To impose the absorbing boundary conditions we need to use 
\be 
M_{\kappa, -\nu}(\zeta) = \frac{\Gamma(1-2\nu)}{\Gamma\left(\frac{1}2- \kappa - \nu\right)} e^{-i \pi \kappa} W_{-\kappa, -\nu}(e^{-i \pi} \zeta) + \frac{\Gamma(1-2\nu)}{\Gamma\left(\frac{1}2 + \kappa - \nu\right)} e^{-i \pi( \kappa + \nu - \frac{1}2)} W_{\kappa, -\nu}( \zeta) \,.
\ee
If we only imposed the regularity at $z \to \infty$ then the mode expansion of $\phi$ would contain four independent creation or annihilation operators:
\be
\phi = \int_0^\infty d\omega \left[c_\omega^\dagger \phi^{\text{in, }(+)}_{-\omega}(x) e^{i \omega t}+ d_\omega^\dagger \phi^{\text{in, }(-)}_{-\omega}(x) e^{i \omega t}+e_\omega  \phi^{\text{in, }(+)}_{\omega}(x) e^{-i \omega t}+ f_\omega  \phi^{\text{in, }(-)}_{\omega}(x) e^{-i \omega t} \right]
\ee
where the normalization of the modes is given by 
\be  
\phi_\omega^{\text{in, }(+)} &= \left(\frac{1}{2\bar \omega}\right)^{1/2} W_{\kappa, -\nu}(\zeta) \nn \\ 
\phi_\omega^{\text{in, }(-)} &= \left(\frac{1}{2\bar \omega}\right)^{1/2} W_{-\kappa, -\nu}(e^{-i \pi}\zeta)   \nn
\ee
and the normalization condition \eqref{eq:normalization-condition} again follows from the property of the Whittaker function, $e^{x}\text{Wr}[\phi_\omega^{\text{in, }(+)}(x)^*, \phi_\omega^{\text{in, }(+)}(x)  ] = i$, where we again note that $\phi_\omega^{\text{in, }(+)}(x)^* = \phi_\omega^{\text{in, }(-)}(x)$. However, if we impose absorbing boundary conditions at the boundary of AdS$_2$ not all operators $b_\omega$, $b_{\omega}^\dagger$, $c_\omega$, $c_\omega^\dagger$ will be linearly independent. Namely, one finds that 
\be 
b_\omega^\dagger = \nn \\
b_{}
\ee

Finally, in the bilocal coordinates we have that 
\be 
(m^2-E^2 q^2) \phi+ \frac{(F(u) - F(\bar u))}{F'(u) F'(\bar u)} \left[-i E q (F'(u) \partial_{\bar u} + F'(\bar u) \partial_u) + (F(u)-F(\bar u)) \partial_u \partial_{\bar u}\right]  \phi =  0
\ee

%%%%%%%%%%%%%%%%%%%%%%%%%%%%%%%%%%%%%%%%%%%%%%%%%%%%%%%%%%%%%%%%%%%%%%%%%%%%%%%%%
\section{Absorption coefficients}

The energy flux is dominated by the $s-$wave and is given by
\be
\frac{d E}{d t} = \int d \omega \frac{\omega\, \sigma_\text{abs}^0}{e^{\beta \omega}-1} = \frac{4 \sqrt{2\pi}}{3} \frac{T^{\frac{3}{2}}}{C^{1/2}}\,, \qquad \text{ for } \qquad T \ll E_{SL(2)}.
\ee
In general, the mode with angular momentum $\ell$ contributes to the energy flux as $T^{3/2 + 2 \ell}$. 

In the microcanonical ensemble Fermi's Golden rule yields, a decay rate
\be
\Gamma_{E_i \to E_i -\omega}=|\cO_{E_i, E_i-\omega}|^2 \rho(E_i-\omega) = \frac{1}{C^{2}} \times  C \sinh\left(2\pi \sqrt{2C(E_i -\omega)} \right)
\ee
which at low final energies becomes 
\be 
\Gamma_{E_i \to E_i -\omega}\sim \sqrt{\frac{E_i-\omega}{C}}
\ee
from which we get 
\be
\frac{dE}{dt} = 
\ee
%%%%%%%%%%%%%%%%%%%%%%%%%%%%%%%%%%%%%%%%%%%%%%%%%%%%%%%%%%%%%%%%%%%%%%%%%%%%%%%%%%%%%%%%%%%%%%%%%%%%%%%%%
\subsubsection*{The pair-production including back-reaction: black holes with smaller charge}

\section{The production of neutral Hawking radiation}

Having computed the rate of Schwinger pair-production, in order to describe how black holes evolve in time when near-extremality, it is equally important to compute the production rate of neutral Hawking radiation when including quantum fluctuations of the metric in the near-horizon region. In \cite{}, the occupation number of Hawking quanta was related to the two-point function of their associated matter field. For simplicity, \cite{} focus on the case of massless radiation. We are interested in the occupation number of Hawking quanta, whose associated Fourier mode is $u_\omega(y) = \frac{1}{\sqrt{4\pi \omega}} e^{-i\omega y}$, seen by an observer that sees the emission process in the vacuum associated to the Poincar\'e frame $F(y) = \tanh \left(\frac{\pi}{\beta} f(y)\right)$. This occupation number can be related to the two-point function in the near-horizon region:
\be 
\label{eq:Nomega-f}
\left(2\pi \delta(0)\right)N_\omega[f] &= -\frac{1}{\pi} \int dy_1 dy_2 u_\omega(y_1) u_\omega^*(y_2) \< \phi(f(u_1)) \phi(f(u_2))\> \nn \\ &=   -\frac{1}{\pi} \int dy_1 dy_2 u_\omega(y_1) u_\omega^*(y_2) \frac{F'(y_1) F'(y_2)}{(F(y_1) - F(y_2))^2}\nn \\ &=   -\frac{1}{\pi} \int dy_1 dy_2 u_\omega(y_1) u_\omega^*(y_2) \frac{f'(y_1) f'(y_2)}{\frac{\beta^2}{\pi^2}  \sinh^2\left(\frac{\pi}{\beta}(f(y_1) - f(y_2))\right)}\,,
\ee
where $f(u)$ parametrizes the large diffeomorphism that captures the fluctuations of the metric in the near-horizon region. The classical solution (that dominates when $T > E_{SL(2)}$) is given by $f(u) = u$, from which \eqref{eq:Nomega-f} gives 
\be 
\label{eq:Nomega-classical}
N_\omega[f(u) = u] = -\frac{1}{2\pi \omega} \int dy_{12} \left(\frac{1}{\frac{\beta}{\pi}\sinh(\frac{\pi}{\beta} y_{12}) }\right)^2 e^{-i\omega y_{12}} =\frac{1}{\pi} \frac{e^{-\frac{\beta \omega}{2}}}{e^{\frac{\beta \omega}2} - e^{-\frac{\beta \omega}2} }\,,
\ee
where we have denoted $t= y_1 - y_2$, where the factor of $1/\omega$ upfront comes from the normalization of $u_\omega(y)$ and 
where to go from the first to the second equality we had to use the $t \to t - i \epsilon$ prescription to go around the double-pole located at $t=0$.\footnote{To obtain this, we can start with the unambiguous Fourier transform formula, 
\be 
\int dt \sech\left(\frac{2\pi}{\beta} t\right)^{2\Delta} e^{i\omega t} = \frac{ 2^{\nu -2 } \beta}{2\pi \Gamma(2\Delta)}  \Gamma\left({\Delta} + i \frac{\omega \beta}{4\pi}\right) \Gamma\left({\Delta} - i \frac{\omega \beta}{4\pi}\right)
\ee
which we use after performing a shift $t \to t + i \frac{\beta}4 - i \epsilon$ we use for $\Delta = 1$.
} (We expect this $\epsilon$-prescription to correspond to the occupation number of emitted, rather than absorbed, particles though I am not yet sure exactly why.) The associated energy flux observed by someone living at the edge of the AdS$_2$ throat is then give by
\be 
\label{eq:energy-flux-classical-result}
\Phi_e^{\text{semi-classical}} = \int_0^\infty d\omega \,\omega \,N_\omega[f(u) = u] = \frac{\pi}{6} {T^2}\,.
\ee

The expectation value of $N_\omega[f]$ when quantum effects become important is then given by 
\be 
\label{eq:exp-value-Nomega}
\<N_\omega \> = \int  DF\, N_\omega[F] \,e^{\frac{T}{E_{SL(2)}}  \int_0^{2\pi} du \Sch(F, u) }\,.
\ee
We can determine the flux directly by integrating \eqref{eq:exp-value-Nomega} against $d\omega \,\omega $. Performing this integral over $\omega$  yields, 
\be 
\Phi_e =  \frac{1}{2\pi} \int dy_{12} \,\delta(y_{12}) \int DF\, \frac{F'(y_1) F'(y_2)}{(F(y_1) - F(y_2))^2}\, e^{\frac{T}{E_{SL(2)}}  \int_0^{2\pi} du \Sch(F, u) }
\ee
where $y_{12} = y_1 - y_2$. Evaluating the two-point function as $y_1 \to y_2$ yields 
\be 
 \frac{F'(y_1) F'(y_2)}{(F(y_1) - F(y_2))^2}  = \frac{1}{y_{12}^2} + \frac{1}{6} \Sch(F, u)\bigg|_{y_1 = y_2 = u } + O(y_{12})\,.
\ee
Subtracting the divergent contact term, we find 
\be 
\label{eq:conf-anomaly-flux}
\Phi_e = \frac{1}{12 \pi} \langle \,\Sch(F, u)\,\rangle = % \frac{1}{12 \pi} \left(2\pi^2 T^2 + \frac{3}2 E_{SL(2)}T\right) 
\frac{\pi T^2}{6} + \frac{1}{8\pi} E_{SL(2)}T\,,
\ee
which at large $T$ matches the classical result but at small $T$ behaves linearly instead. 

We can also determine $N_\omega$ exactly. We can start by woking in the microcanonical ensemble. In such a case the occupation number can be written as, 
\be 
\label{eq:occupation-number}
\langle E|\omega N_\omega | E \rangle = \frac{1}{4\pi} \left( \rho(E +\omega) |\cO_{E, E+\omega}^{1}|^2 + \frac{1}{4\pi} \rho(E-\omega) |\cO_{E, E-\omega}^{1}|^2 - \rho(\omega) |\cO_{0, 0+\omega}^{1}|^2 - \rho(-\omega) |\cO_{0, 0-\omega}^{1}|^2  \right)
\ee
where
\be 
|\cO_{E_1,E_2}^{\Delta}|^2 = \frac{\Gamma(\Delta \pm i\sqrt{E_1}\pm i\sqrt{E_2})}{\Gamma(2\Delta)}\,,
\ee
and,
\be 
\rho(E)= \frac{1}{2\pi} \sinh\left(2\pi \sqrt{\frac{E}{E_{SL(2)}}}\right)
\ee 
Above, $E$ should be identified as the energy above extremality that the black hole has before absorbing/emitting a photon. 
The way I see it, the meaning of the first term is that the black hole gains energy when absorbing a photon, while the meaning of the second term is that of the black hole losing energy when emitting a photon. We will therefore call them the emitting and absorbing branches. The last two terms calibrate the density of states to be vanishing when $E=0$ and $\omega =0$.  We plot the real and imaginary part of the first and second term in figure~\ref{fig:Nomega}. Notice that the emitting curve has an imaginary occupation number for $\omega > M$ -- this is of course to be expected since the black hole cannot emit photons with energy larger than their mass. The absorbing branch is purely real since the black hole can absorb photos with any energy. 

Integrating \eqref{eq:occupation-number} to find the flux we get figure~\ref{fig:Nomega}. Summing up the two branches we get a flux consistent with the conformal anomaly result -- the numerical integral is shown by the blue dots, while the analytic result  
\be
\label{eq:total-flux}
\Phi_\gamma^{\text{total}}(E) = \int_0^\infty d\omega \, \Re \left(\omega N_\omega\right) = \frac{E_{SL(2)} E}{12 \pi} \left(1+ O\left(\frac{E}{E_{SL(2)}}\right)\right)\,,
\ee 
is shown by the blue straight line. However, one might choose to solely keep the emitting branch if we are interested in an observer whose goal is solely to detect emitting radiation. If we are interested in the flux obtained from this branch alone in the strongly-coupled limit we have, 
\be 
\label{eq:emitted-flux}
\omega N_\omega &= \frac{\sqrt{E_{SL(2)}(E-\omega)}}{4\pi^2} \left(1+ O\left(\frac{E}{E_{SL(2)}}\right)\right)\,, \nn \\  \Phi_{\gamma}^\text{emit.} &= \int_0^M d\omega \, \omega N_\omega = \frac{E_{SL(2)}^{1/2}E^{3/2}}{6\pi^2} \left(1+ O\left(\frac{E}{E_{SL(2)}}\right)\right)\,,
\ee 
which should be contrasted with the linear behavior of the total flux obtained from the conformal anomaly in \eqref{eq:conf-anomaly-flux} or with \eqref{eq:emitted-flux}. 
\LVI{We should discuss what we think is the correct result at this point.}]

\begin{figure}
    \centering
    \includegraphics[width=0.49\textwidth]{ReomegaNomega.pdf}
     \includegraphics[width=0.49\textwidth]{ImomegaNomega.pdf}
    \caption{The real and imagianry parts of the occupation number for $M=1/10$ and $E_{SL(2)} = 1$. The green represent the absorbing branch while the red is the emitting branch while the blue curve is the total occupoation number.}
    \label{fig:Nomega}
\end{figure}

\begin{figure}
    \centering
    \includegraphics[width=0.49\textwidth]{flux.pdf}
    \caption{The real and imagianry parts of the occupation number for $M=1/10$ and $E_{SL(2)} = 1$. Again the contribution of the emitting branch is shown in red, while that of the absorbing branch is shown in green. }
    \label{fig:Nomega}
\end{figure}

We can now translate these results to the canonical ensemble. Using the exact formula for the two-point function of fields in the presence of metric fluctuations \eqref{eq:exp-value-Nomega} becomes:
\be 
\label{eq:exp-value-Nomega-interm-formula}
\<N_\omega \> = \frac{1}{\pi^3 \omega}\int dt e^{-i\omega t} \int d\mu(k_1) d\mu(k_2) |\cO^1_{k_1^2, k_2^2}|^2 e^{-\beta k_2^2  - it (k_1^2 - k_2^2)}\,,
\ee
where 
\be 
\label{eq:measure-integral-over-energies}
d\mu(k) = dk \frac{k}{E_{SL(2)}}  \sinh\left(2\pi \frac{k}{\sqrt{E_{SL(2)}}}\right)\,.
\ee
In \eqref{eq:exp-value-Nomega-interm-formula}, $E_1= k_1^2$ and $E_2=k_2^2$ should be interpreted as the energies of the black hole before and after the emission process, respectively. Above, $\Gamma(1\pm ik_1\pm ik_2)$ is a short-hand for the product of four-gamma functions with all possible sign combinations. If $\beta E_{SL(2)}$ is large, then \eqref{eq:exp-value-Nomega-interm-formula} can be evaluated by saddle-point and the result is precisely \eqref{eq:Nomega-classical}.  The integral over $t$ enforces that $k_2^2 = k_1^2 + \omega$ as expected from energy conservation. Thus, we find that 
\be 
\label{eq:exp-value-Nomega-final-formula}
\<N_\omega \> = \frac{1}{\pi^3 \omega Z(\beta)} \int dk \,k\, \sinh\left(2\pi \frac{k}{\sqrt{E_{SL(2)}}}\right) \sinh\left(2\pi \sqrt{ \frac{k^2+\omega}{E_{SL(2)}}}\right) |\cO^1_{ k^2+\omega,k^2}|^2 \,e^{-\beta (k^2  + \omega)}\,,
\ee
where we can now identify $E=k^2+\omega$ with the energy that the black hole had initially above extremality and $k^2$ with the energy above extremality after the emission occurs. We are most interested in evaluating the integral in the regime where $\beta E_{SL(2)}$ is small. In such a case, if we scale $\beta \sim 1/\epsilon$ (where $\epsilon$ is a small proxy parameter that is useful for bookkeeping purposes), then \eqref{eq:exp-value-Nomega-interm-formula} should be dominated by energies with $k \sim O(\sqrt{\epsilon})$ and the resulting $N_\omega$ should largely have non-zero support on frequencies $\omega \sim O(\epsilon)$. In such a limit, \eqref{eq:exp-value-Nomega-final-formula} becomes 
\be
\<N_\omega \> = \frac{4}{\pi \omega Z(\beta)} \int dk \, \frac{k^2 \sqrt{k^2 +\omega}}{E_{SL(2)}^2} e^{-\beta (k^2+\omega)} =  \frac{\beta^{\frac{1}2}e^{-\frac{\beta \omega}2} K_1\left(\frac{\beta \omega}2\right) }{2\pi E_{SL(2)}^2}\,.
\ee
The overall observed energy flux is then given by 
\be 
\label{eq:quantum-corrected-flux}
\Phi_\gamma^\text{emit.} = \int_0^\infty d\omega \,\omega\, \<N_\omega \> =  \frac{4 \pi^2}{3} \left({T^{\frac{3}2}}{E_{SL(2)}}^{\frac{1}{2}}\right) \qquad \text{ when } \qquad \frac{T}{E_{SL(2)}} \ll 1\,,
\ee
which again scales with the power of $3/2$ instead of the semi-classical result which is a square of the temperature or the total flux which is linear in $T$. 
%%%%%%%%%%%%%%%%%%%%%%%%%%%%%%%%%%%%%%%%%%%%%%%%%%%%%%%%%%%%%%%%%%%%%%%%%%%%%%%%%%%%%%%%%%%%%%%%%%%%%%%%%%%%%%%%%%%%%%%%%%%%%%%%%
%%%%%%%%%%%%%%%%%%%%%%%%%%%%%%%%%%%%%%%%%%%%%%%%%%%%%%%%%%%%%%%%
\section{Schwinger pair production}

We will work in the S-wave sector which allows us to make the following ansatz about the metric, 
\be 
\label{eq:ansatz-for-the-metric}
ds^2 = \frac{r_0}{\Phi^{1/2}} g_{\mu\nu} + \Phi d\Omega_{S^2}
\ee
where $\Phi$ is the dilaton field that parametrizes the transverse area of $S^2$ and $g_{\mu \nu}$ is the $2d$ metric. The factor $\frac{r_0^{1/2}}{\Phi^{1/2}}$ is conveniently chosen such that when dimensionally reducing the Einstein-Maxwell action using the ansatz \eqref{eq:ansatz-for-the-metric}, no kinetic term is produced for $\Phi$. After integrating out the gauge field when working in the canonical ensemble where the boundary field strength is fixed (such that the electric flux is associated to an overall charge $Q$) we have, 
\begin{align}
\label{eq:total-action}
I_{\rm total}[g,\Phi]\;\;&=\;\;-\frac{1}{4G_{N}}\int_{M_{\rm interior}}d^{2}x\sqrt{g}\:[\Phi R-2U_{Q-q}(\Phi)] + m \int_{\partial M_{\rm interior}} du \sqrt{\frac{r_0}{\Phi^{1/2}}g_{\mu \nu} \dot x^{\mu} \dot x^{\nu}} \nonumber \\ 
&-\frac{1}{4G_{N}}\int_{M_{\rm outside}}d^{2}x\sqrt{g}\:[\Phi R-2U_{Q}(\Phi)] - \frac{1}{2G_N} \int_{\partial M_{\rm outside}} du \sqrt{h} \Phi K
\end{align}
where $Q-q$ can be identified as the new charge of the black hole, while $q$ and $m$ are the charge and mass of the particle respectively. $M_{\text{interior}}$ is the geometry within the charged instanton; $M_{\text{outside}}$ is the geometry outside of the instanton region whose asymptotic boundary is $\partial M_{\rm outside}$. The dilaton potential $U_{Q}(\Phi)$ is given by, 
\be
U_{Q}(\Phi)~~=~~r_{0}\left[\frac{G_N}{4\pi}\frac{Q^2}{\Phi^{3/2}}-\frac{1}{\Phi^{1/2}}\right]
\ee
The variation of such an action is given by, 
\begin{align}
\label{eq:total-action-variation}
    \delta I_{\rm total}[g, \Phi] &= EOM_{\rm interior } + EOM_{\rm outside} - \frac{1}{4G_N} \int_{\partial M_{\rm outside}} du ([2(\partial_n \Phi - \Phi K)] \delta(\sqrt{g_{uu}}) - 2 \Phi \sqrt{g_{uu}} \delta K)  \nonumber \\
    & - \frac{1}{2 G_N} \int_{\partial M_{\rm outside}} du \sqrt{h} \Phi \delta K +  \frac{1}{4G_N} \int_{\partial' M_{\rm outside}} du ([2(\partial_n \Phi - \Phi K)] \delta(\sqrt{g_{uu}}) - 2 \Phi \sqrt{g_{uu}} \delta K)  \nonumber \\ 
    & -   \frac{1}{4G_N} \int_{\partial M_{\rm interior}} du ([2(\partial_n \Phi - \Phi K)] \delta(\sqrt{g_{uu}}) - 2 \Phi \sqrt{g_{uu}} \delta K) +  m \int du \frac{r_0^{1/2}}{\Phi^{1/4}} \left( \delta(\sqrt{g_{uu}}) - \sqrt{g_{uu}} \frac{\delta \Phi}{4\Phi}\right)  
\end{align}
where $\partial M_{\text{interior}}$, $\partial' M_{\text{outside}} $ and $\partial M_{\text{outside}}$ are the boundary of the instanton region measured from the inside, from the outside or the asymptotic boundary of the entire geometry, respectively. Above, the induced boundary metrics used in \eqref{eq:total-action-variation} are given by 
\be 
g_{uu} = g_{\mu \nu} \dot x^\mu \dot x^{\nu}|_{\partial M_{\text{outside}} \text{ or } \partial M_{\text{outside}} \text{ or } \partial M_{\text{interior}}} \,.
\ee
If imposing Dirichlet boundary conditions on the outside boundary (fixed BH temperature and fixed size of the transverse $S^2$), then the boundary terms on $\partial{M_{\text{outside}}}$ in the variation of \eqref{eq:total-action-variation} vanishes. We are left with solving the EOM$_{\text{interior}}$ and EOM$_{\text{outside}}$ as well as the variation along the boundary of the instanton. The solution for the former two are given by: 
\begin{align}
\,,\nn \\ 
\text{Interior}: \qquad \Phi(\bar r) = \bar r^2. \qquad ds^2 = \frac{\Phi^{1/2}}{r_0} \left[\bar\chi^2(\bar r) d\bar\tau^2 + \frac{d \bar r^2}{\bar \chi(\bar r)^2}\right], \qquad \bar \chi(\Phi)^2 =1+ \frac{G_N}{4\pi}\frac{\bar Q^2}{\Phi} - \frac{ 2 G_N \bar M}{\Phi^{1/2}} \nn \\
\text{Outside}: \qquad \Phi( r) =  r^2 \qquad ds^2 = \frac{\Phi^{1/2}}{r_0} \left[\chi^2(r) d \tau^2 + \frac{d  r^2}{ \chi( r)^2}\right]\,,\qquad \chi(\Phi)^2 =1+ \frac{G_N}{4\pi}\frac{Q^2}{\Phi} - \frac{2 G_N M}{\Phi^{1/2}}
\end{align}
where $\bar Q = Q-q$ and $M$ and $\bar M$ are, so far, two undetermined constants. We can also rescale time in the inside of the instanton such that, $\bar \tau=A \tau$. The continuity condition which says that the proper length of the instanton boundary has to be the same when measured from the inside/outside is: 
\be 
\label{eq:cont-criterion}
A \bar \chi = \chi\,.
\ee

Additionally, setting the variation of the boundary terms on $\partial' M_{\text{outside}} + \partial M_{\text{interior}}$ to vanish we find:
\begin{align}
\delta K&: \qquad \Phi|_{\partial M_{\text{outisde}}} = \bar \Phi|_{\partial M_{\text{inside}}} \Rightarrow r=\bar r=r_\inst\,,\nn \\ 
\delta \Phi&: \qquad \Delta K = \frac{m r_0^{1/2}}{\Phi^{5/4}} \Rightarrow \,\, \Delta K_{\tau\tau} = \frac{m r^{5/2}}{r_0^{1/2}} \Rightarrow \frac{1}{\chi} \left( M-
\frac{Q^2}{r_\inst}\right) - \frac{1}{\bar \chi} \left(\bar M- \frac{\bar Q^2}{r_\inst} \right) = m \nn \\ 
\delta \sqrt{g_{uu}}&:\qquad \frac{1}{4} \Delta \left(2\partial_n \Phi - 2\Phi K \right ) = -m \frac{r_0^{1/2}}{\Phi^{1/4}} \Rightarrow \Delta( \partial_n \Phi) =  - m \frac{r_0^{1/2}}{r^{1/2}}\Rightarrow r_\inst \left(\chi-\bar \chi\right)  = -m\,.
\label{eq:variation-boundary}
\end{align}

\begin{figure}
    \centering
    \includegraphics[width=0.6\textwidth]{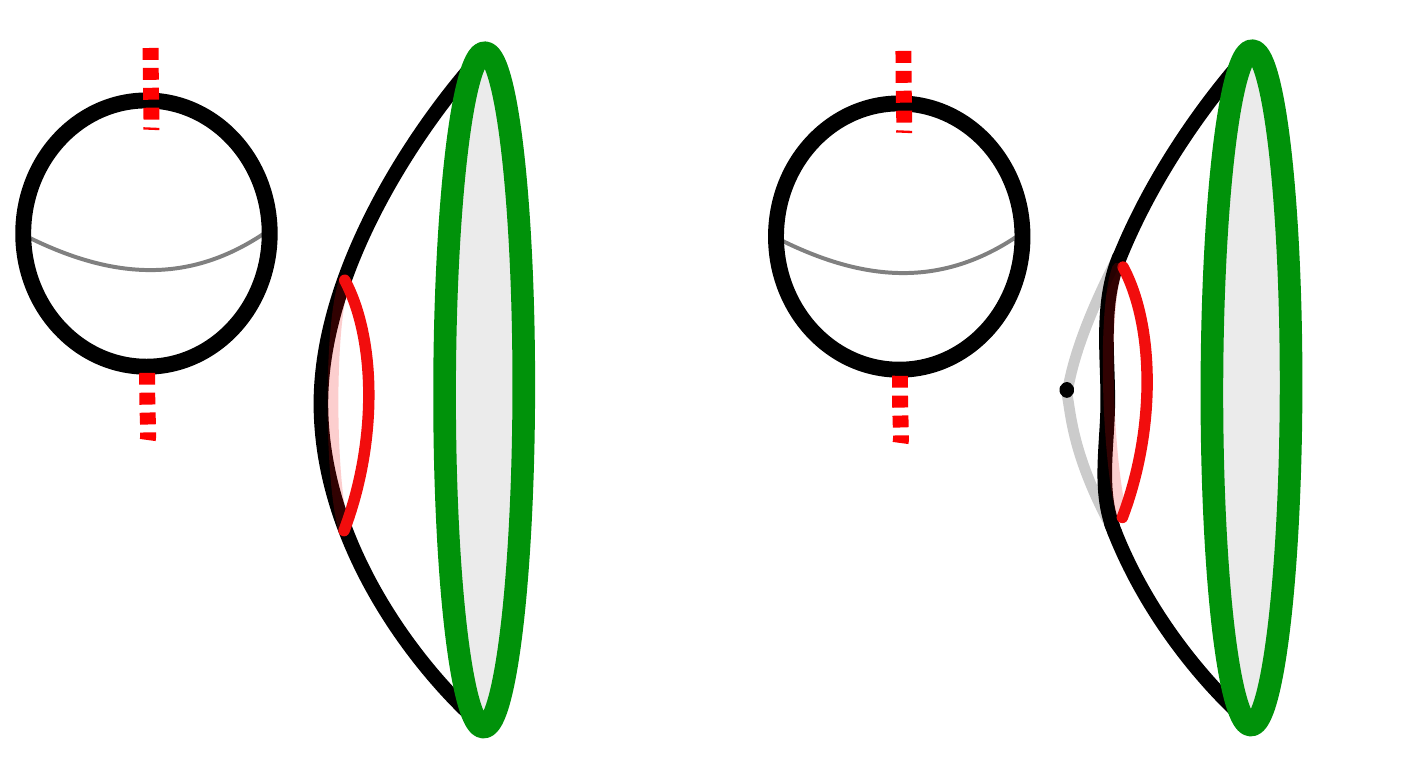}
    \caption{Instanton configuration in the near-horizon AdS$_2 \times S^2$ region of a near-extremal black hole. The effect of the backreaction is captured by the difference between the left and right figures - while both geometries are smooth, for the geometry on the right if we hypothetically continue the spacetime past the location of the charged particle we see that the resulting geometry has a very blunt defect whose angle is $2\pi \alpha$, with $\alpha$ given by \eqref{eq:defect-angle}. We represent the location of the defect through the dotted point.   }
    \label{fig:Nomega}
\end{figure}

Finally, we indeed want to derive period of $\tau$ (with $\tau \sim \tau + \beta_\text{corr}$) from imposing that the region inside the instanton is smooth. This yields, 
\be 
\label{eq:smoothness-inside-inst}
\beta_\text{corr} = \frac{2\pi}{A} \frac{2\bar r^2_+}{\bar r_+ - \bar r_-} 
\ee
where $\bar r_\pm = \bar M \pm \sqrt{\bar M^2 - \bar Q^2}$ are the locations of the inner and outer horizon inside of the instanton. We should remember that $ \beta_\text{corr}$ and $Q$ are the quantities we keep fixed, while $M$, $\bar M$, $A$ and $r_\text{inst}$ are the quantities that we solve for from the continuity criterion \eqref{eq:cont-criterion}, the variation on the boundary of the instanton \eqref{eq:variation-boundary}, and the smoothness of the inside of the instanton geometry \eqref{eq:smoothness-inside-inst}. All these equations can be solved and one important quantity that we are looking for is the defect angle that occurs if continue the outside geometry past the instanton. Imagining doing that and expanding around the Euclidean horizon of this imagined geometry we have
\be
ds^2 = dx^2 + \frac{(r_+-r_-)^2}{r_+^2} x^2 d\tau^2+\dots
\ee
the defect angle would be given by 
\be 
\label{eq:defect-angle-intro}
\alpha= \frac{ \beta_\text{corr}}{\beta} \,,\qquad \text{ where }\qquad \beta = 2\pi \frac{2r_+^2}{r_+-r_-}\,.
\ee
Solving the equations, one find 
\be
\label{eq:defect-angle}
\alpha= \frac{\bar r_+^2}{r_+^2} = \frac{\left(\sqrt{(2Q-q)^2 - m^2} + \sqrt{q^2-m^2}\right)^4}{16Q^2} = 1-2\frac{q-\sqrt{q^2-m^2}}{Q} + O\left(\frac{1}{Q^2}\right)
\ee
where in the last step we have taken the limit in which $Q \gg q$. 

\begin{figure}
    \centering
    \includegraphics[width=0.5\textwidth]{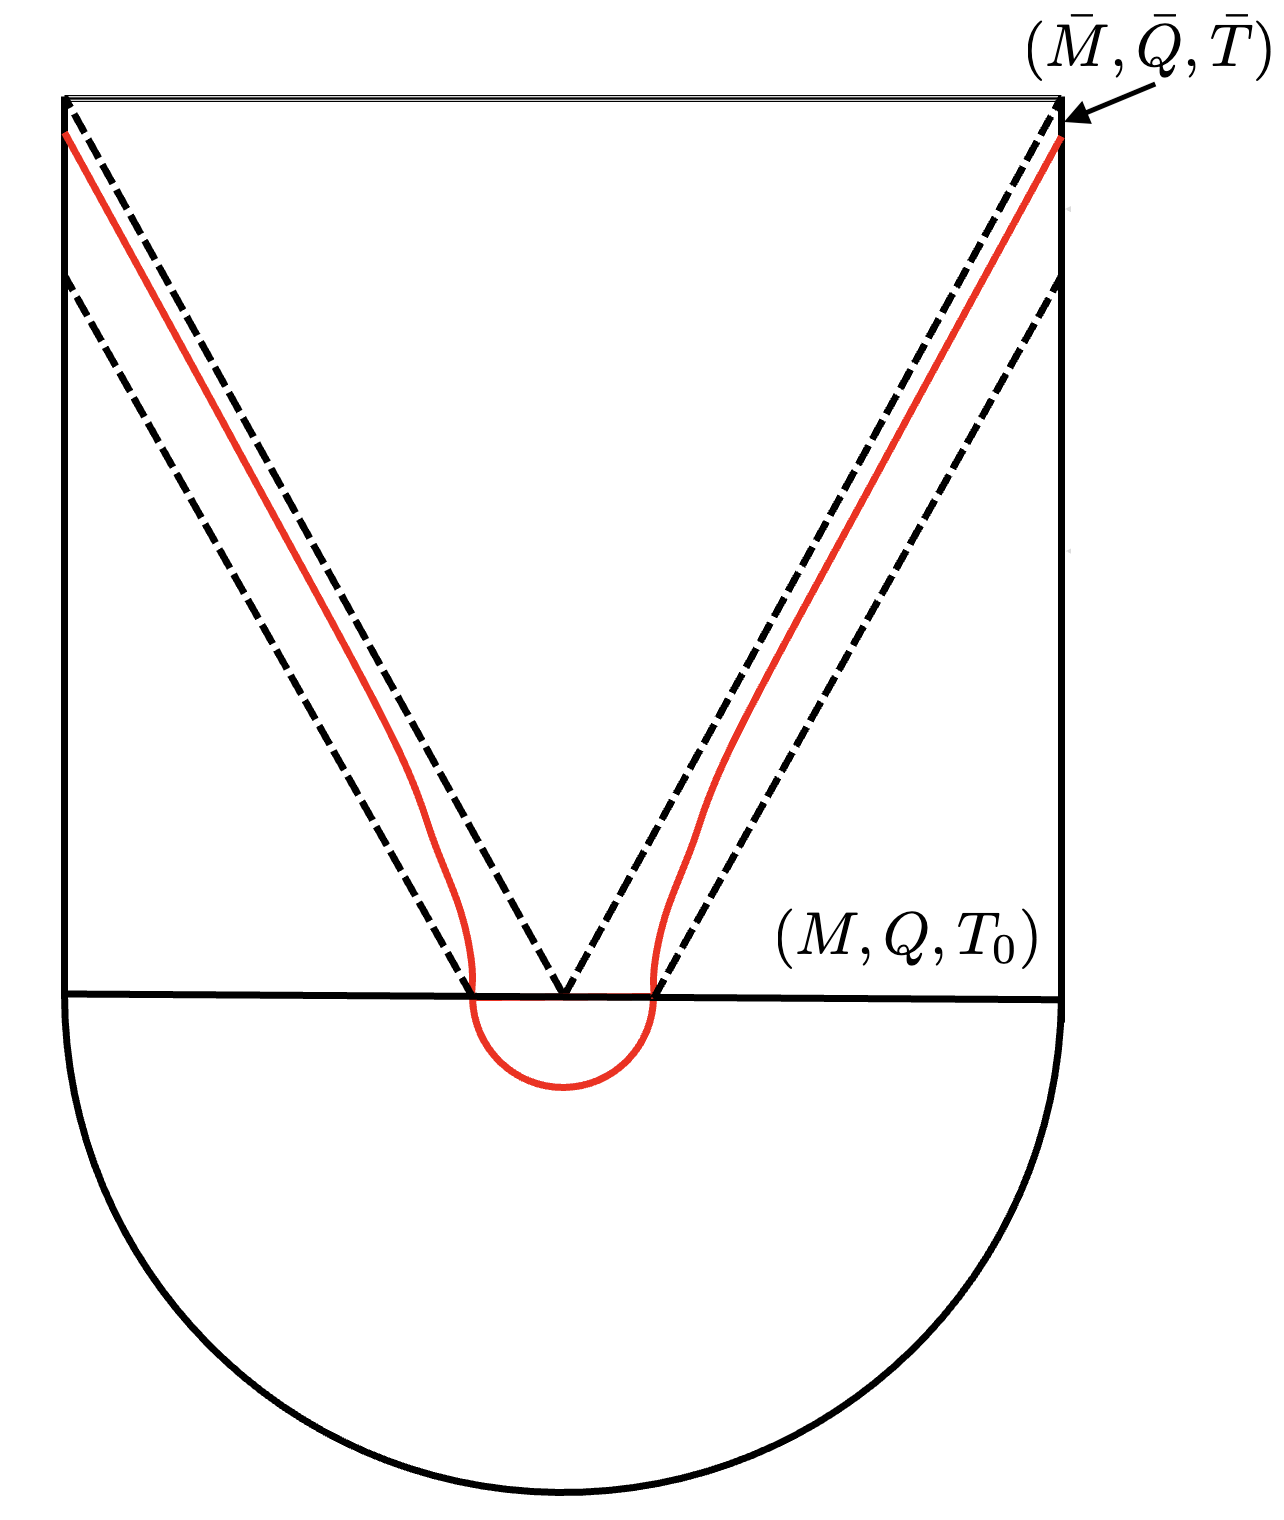}
    \caption{Instanton configuration when analytically continuing the geometry to Lorentzian signature. We point out the temperatures $T$, $T_\text{corr}$ and $\bar T$ that an observer would detect at various times.  }
    \label{fig:Nomega}
\end{figure}

It is also useful to keep track of the mass $\bar M$. This can be viewed as the final ADM mass obtained after the expelled charged particle reaches the observer. This can be found to be 
\be 
\label{eq:barM-exact-formula}
\bar M = \frac{\sqrt{q^2-m^2} \sqrt{(M-Q) (M+Q)} \sqrt{(q-2 Q)^2-m^2}+ M (q^2-m^2-2q Q+ Q^2)}{2 Q^2}\,,
\ee
where we can think about the initial mass $M$ as that of a black hole of charge $Q$ and inverse-temperature $\beta$ (not $\beta_\text{corr}$). To get some intuition about $\bar M$ consider the evaporation process in which the black hole has an initial temperature $T \ll E_{SL(2)}$. Then, to leading order in $T$ we find 
\be 
\label{eq:barM-smallT-largeQ}
\bar M = \bar Q + \frac{q^2-m^2}{2Q} + O(T)  =  Q-q + \frac{q^2-m^2}{2Q} + O(T) \,,
\ee
where it is important to note that, for sufficiently large black holes, we always have that $ \frac{q^2-m^2}{2Q} \gg E_{SL(2)}\sim \frac{1}{Q^3}$. 
There are two things to note. (i) The mass $\bar M$ is wildly different than $M-m \approx Q - m$, which implies that the charged particle has very high energy by the time it reaches the observer. (ii)  As long as we start with a sufficiently cold black hole,  the resulting temperature after emission will be largely independent of the temperature before emission and, for sufficiently large black holes, they will always bring the mass of the black hole above the $E_{SL(2)}$ thermodynamic breakdown scale. The final temperature, which we will denote by $\bar T$ (and inverse by $\bar \b$) can also be computed from the initial temperature as, 
\be 
\label{eq:barT}
\bar T = \frac{T}{\alpha A} = \frac{T_\text{corr}}{A}\,,
\ee
with $\alpha$ given by \eqref{eq:defect-angle} and $A$ given by 
\be 
A = \sqrt{\frac{M^2-Q^2}{\bar M^2- \bar Q^2}}
\ee
which can be obtained exactly from \eqref{eq:barM-exact-formula} and  remembering that $\bar Q = Q-q$. If working with a black hole which has a small initial  temperature, whose charge $Q\gg q$, then $\bar T$ indeed agrees with the prediction from \eqref{eq:barM-smallT-largeQ} and is given by 
\be 
\label{eq:barT-leading-in-T}
\bar T  = \frac{\sqrt{q^2-m^2},}{2\pi Q^2} + O\left(T,\,\frac{1}Q\right)\,.
\ee

%%%%%%%%%%%%%%%%%%%%%%%%%%%%%%%%%%%%%%%%%%%%%%%%%%%%%%%%%%%%%%%%%%
\subsection{Single instanton}

The instanton action is given by 
\be 
I_\text{inst + BH} = \pi r_+^2
\ee
Expanding at large $Q$ we find 
\be 
\label{eq:1-inst-contribution}
I_\text{inst + BH} = - \pi \bar r_+^2  &= -\pi Q^2 + 2\pi Q \left(q - \sqrt{q^2-m^2} \right)  \nn \\ &- \frac{8\pi^2 Q^3}{\beta} \left(1 - 4\frac{q + \sqrt{m^2 - q^2}}Q \right) + O\left(\frac{1}{Q^2}, \, \frac{\pi^2 Q^6}{\beta^2}\right)
\ee
Note that this can be written as, 
\be 
I_\text{1 inst + BH} = - \pi \bar r_+^2  &= -\pi Q^2 + 2\pi Q \left(q - \sqrt{q^2-m^2} \right)  \nn \\ &- \frac{8\pi^2 Q^3}{\beta} \alpha^2 + O\left(\frac{1}{Q^2}, \, \frac{\pi^2 Q^6}{\beta^2}\right)
\ee 
where the last term can be identified as the on-shell contribution of the Schwarizan with a defect (with angle $\alpha$). This in fact holds outside of a $1/Q$ expansion and only in a $1/\beta$ expansion. 

Using the quantization of the theory with a defect angle $\alpha$, the partition function of the BH and instanton system can be written as, 
\begin{align}
Z_{BH+1\,\inst} &=   \underbrace{\left[ i Z_{\text{1-loop particle}} e^{- 2\pi Q \left(q - \sqrt{q^2-m^2} \right)} \right]}_{\substack{\text{Contribution of non-interacting}\\ \text{ charged particle}}} \underbrace{\left(\frac{Q^3}{\beta}\right)^{1/2}}_{\substack{\text{Gravitational}\nn \\\text{ one-loop determinant}}} \,   \exp\underbrace{\left[{\pi Q^2 + \frac{8\pi^2 Q^3}{\beta} \alpha^2 }\right]}_{\substack{\text{Classical grav. contribution }\\ \text{including backreaction}} }\\ &\times \underbrace{Q^\#}_{\text{Other one-loop det.'s}}\left(1+O(1/Q)\right)\,,
\label{eq:BH+1-inst-part-function}
\end{align}
where $i Z_{\text{1-loop particle}} $ is the one-loop contribution of the particle moving in AdS$_2$ excluding the translation and rotation modes that are already taken into account by Schwarzian. In appendix \ref{app:one-loop-det-particle-in-AdS} we find this to be 
\be
Z_{\text{1-loop particle}} = 
\frac{1}{8\pi^3}\left(2\pi Q \sqrt{q^2-m^2-\frac{1}{4 Q^2}} - 1\right)
\ee 
The $\left(\frac{Q^3}{\beta}\right)^{1/2}$ factor in \eqref{eq:BH+1-inst-part-function} is the contribution of the graviton one-loop determinant. Finally, the quantity in the exponent is the corrected black hole on-shell action. 

The partition function with an instanton should be compared to the BH partition function for which
\be 
Z_{BH} = \underbrace{Q^\#}_{\text{Other one-loop det.'s}}  \underbrace{\left(\frac{Q^3}{\beta}\right)^{3/2}}_{\substack{\text{Gravitational}\\\text{ one-loop determinant}}} \,   \exp\underbrace{\left[{\pi Q^2 + \frac{8\pi^2 Q^3}{\beta}  }\right]}_{\substack{\text{Classical grav. contribution }\\ \text{including backreaction}} }
\ee
Note that the graviton one-loop determinants in the two calculation are different. This is because the isometries of the two geometries are also different: the near-horizon of a BH has an $SL(2, \mR)$ isometry, while the BH with an instanton breaks that isometry to $U(1)$. The different powers of $\beta^{-1/2}$ simply count the number of gravitational modes that we do not integrate over; since we should not integrate over the fluctuations generating an isometry transformation the two geometries consequently have different one-loop determinants.  We find that the ratio of the two partition functions is given by 
\be 
\label{eq:ratio-of-two-partition-function}
\frac{Z_{BH+1\,\inst}}{Z_{BH} } = \frac{\beta}{Q^3}  \left[ i \underbrace{Z_{\text{1-loop particle}} e^{- 2\pi Q \left(q - \sqrt{q^2-m^2} \right)}}_{\equiv e^{-I_{\inst \text{ eff.}}}} \right] \exp\left[{\frac{8\pi^2 Q^3}{\beta}  } (\alpha^2-1)\right]
\ee
which gives us a first estimate for the decay rate in a regime where $\frac{Z_{BH+1\,\inst}}{Z_{BH} } \ll 1$, i.e.~when $\beta/Q^3 \ll e^{I_{\inst \text{ eff.}}}$,  
\be 
\Gamma = \frac{1}\beta \Im \, \log \, \left(1+\frac{Z_{BH+1\,\inst}}{Z_{BH} }\right) =_{\frac{Z_{BH+1\,\inst}}{Z_{BH} } \ll 1}  \frac{1}{Q^3} Z_{\text{1-loop particle}} e^{-I_{\inst \text{ eff}} + {\frac{8\pi^2 Q^3}{\beta}  } (\alpha^2-1)}\,.
\ee

\subsection{Single winding instanton}

We now considering a particle that winds $k$ times around its circular trajectory. This amounts to sending $m \to k\, m$ and $q \to k \,q$. Therefore, the defect angle becomes 
\be
\label{eq:alpha-k}
\alpha_k =  \frac{\left(\sqrt{(2Q-k q)^2 - (km)^2} + k\sqrt{q^2-m^2}\right)^4}{16Q^2} = 1-2k\frac{q-\sqrt{q^2-m^2}}{Q} + O\left(\frac{1}{Q^2}\right)\,,
\ee 
where the latter expression is valid as long as $k q \ll Q$. The on-shell action is given by 
\be 
I_\text{1 inst + BH}  &= -\pi Q^2 + 2\pi k Q \left(q - \sqrt{q^2-m^2} \right)  - \frac{8\pi^2 Q^3}{\beta} \alpha_k^2 + O\left(\frac{1}{Q^2}, \, \frac{\pi^2 Q^6}{\beta^2}\right)\,.
\ee 
Finally, accounting for the one-loop determinant whose computation we reviewed in appendix \ref{app:one-loop-det-particle-in-AdS}, we find the effective action of the $k$-times winding instanton to be  
\be 
\label{eq:inst-eff-k}
e^{-I_\text{inst eff.}^{k}} = \frac{(-1)^k }{ k^2} \left(1-2\pi k Q \sqrt{q^2-m^2-\frac{1}{4 Q^2}} \right) e^{ -2\pi k Q \left(q - \sqrt{q^2-m^2} \right)}
\ee
We will use this result below in order to be able to find the full pair-production rate when also including multi-instanton contributions.
\subsection{Multi-instanton contribution}
\label{sec:multi-instanton-cont}

To get the contribution of all instantons we have to account for the volume of the multi-defect moduli space on hyperbolic geometries. The partition function with an arbitrary number of defects was found to be related to the KdV couplings in the minimal string equation in the $(2,p)$ minimal model. These KdV couplings $t_k$ are captured by the function  
\be 
\mathcal F(u) = \sum_k t_k u^k\,. 
\ee
$\cF(u)$ is related to the density of states associated to the partition function that we are looking for through 
\be 
\label{eq:density-of-states-from-F}
\rho(E) = \frac{e^{\pi Q^2}}{2\pi E_{SL(2)}} \int_{2 \gamma E_0 \equiv u(0)}^{2 \gamma E}  \frac{du}{\sqrt{2 \gamma E-u}} \frac{\partial \cF}{\partial u}\,,
\ee
where we have defined $\gamma = E^{-1}_{SL(2)}$, which finally gives the partition function 
\be 
Z_\text{sum over defects}(\beta) = \int_{E_0}^\infty dE \rho(E) e^{-\beta E}\,. 
\ee
We will assign defects with a weight given by 
\be 
e^{-I_\text{inst eff}} = Z_\text{1-loop particle} \,e^{\frac{\pi}{16Q^2} \left[\left(\sqrt{(2Q-q)^2-m^2} +\sqrt{q^2-m^2}\right) - 16 Q^4\right] }\,,
\ee
which is associated to the instanton of each defect whose angle is $\alpha$ from \eqref{eq:defect-angle}. This is for the dominant instantons with $k=1$. In addition to this, there are also suppressed instantons that wind $k$-times whose weight will be given by $
e^{-I_\text{inst eff.}^{k}} $ from \eqref{eq:inst-eff-k} whose associated angle is $\alpha_k$ from \eqref{eq:alpha-k}. Note that all the defect actions as well as the defect angle are independent from the number of defects that we put on the black hole background. 

To start we will neglect the contribution of winding instantons. In such a case $\cF(u)$ was found to be given by a trunated sum
\be
\label{eq:F(u)-exact}
\cF(u) = \sum_{L=0}^{\left\lfloor \frac{1}{1-\alpha}\right\rfloor} \frac{i^L e^{-L I_\text{inst eff}}}{L!} \left(\frac{2\pi(1-L(1-\alpha))}{\sqrt{u}}\right)^{L-1} I_{L-1}\left(2\pi(1-L(1-\alpha)) \sqrt{u}\right) 
\ee
where $I_{L-1}(x)$ are Bessel functions. This sum can be conveniently rewritten in terms of a generating function:
\be 
\label{eq:F(u)-generating-function}
\mathcal F(u) = \int_\mC \frac{dy}{2\pi i} e^{2\pi y} \left(y-\sqrt{y^2 - u - 2 i e^{-I_\text{inst eff}} e^{-2\pi(1-\alpha)y} }\right)
\ee
A similarly useful formula is that of the generating function for the density of states, which is given by 
\be 
\label{eq:density-of-states-generating-function}
\rho(E) = \frac{e^{\pi Q^2}}{2\pi E_{SL(2)}} \int_\mC \frac{dy}{2\pi i} e^{2\pi y} \tanh^{-1}\left(\sqrt{\frac{2 \gamma \left(E-E_0\right)}{y^2-2  i e^{-I_\text{inst eff}} e^{-2\pi(1-\alpha)y} - 2 \gamma E_0}}\right)\,.
\ee
The generating functions \eqref{eq:F(u)-generating-function} and \eqref{eq:density-of-states-generating-function} can now be generalized to include $k$-times winding instantons:
\begin{align}
\label{eq:generating-function-including-k-times-winding}
\mathcal F(u) &= \int_\mC \frac{dy}{2\pi i} e^{2\pi y} \left(y-\sqrt{y^2 - u - 2 i \sum_{k=1}^\infty e^{-I_\text{inst eff}^k} e^{-2\pi(1-\alpha_k)y} }\right)\,,\nn \\ 
\rho(E) &= \frac{e^{\pi Q^2}}{2\pi E_{SL(2)}} \int_\mC \frac{dy}{2\pi i} e^{2\pi y} \tanh^{-1}\left(\sqrt{\frac{2 \gamma \left( E-E_0\right) }{y^2- 2 \gamma E_0-2  i \sum_{k=1}^\infty e^{-I_\text{inst eff}^k} e^{-2\pi(1-\alpha_k)y} }}\right)\,.
\end{align}

\subsubsection*{A sanity check: reproducing the pair-production rate without backreaction}

As a sanity check, we can first see what happens in the complete absence of backreaction in which case we are neglecting the presence of defects, which implies we are taking $\alpha =1$ and keeping $e^{-I_\text{inst eff}
}$ as in \eqref{eq:ratio-of-two-partition-function}: 
\be
\cF(u) = \sum_{L=0}^{\infty} \frac{i^L e^{-L I_\text{inst eff}}}{L!} \left(\frac{2\pi}{\sqrt{u}}\right)^{L-1} I_{L-1}\left(2\pi \sqrt{u}\right)= \frac{\sqrt{u+2i e^{-I_\text{inst eff}}}}{2\pi} I_{1}\left(2\pi \sqrt{u+2i e^{-I_\text{inst eff}}} \right)\,.
\ee
where one identifies the second expression as the infinite Taylor serier in $i e^{-I_\text{inst eff}}$ of the third expression. The edge of the spectrum in such a case is given by 
$2 \gamma E_0 = -2 i e^{-I_\text{inst eff}}$, the density of states is found to be 
\be
\rho_\text{no backreaction}(E) \sim \frac{e^{\pi Q^2}}{E_{SL(2)}}\sinh\left(2\pi \sqrt{2 \gamma \left( E-E_0\right)} \right)
\ee
which consequently gives a partition function 
\be 
Z_\text{no backreaction} = Z_{BH} e^{-\beta E_0}  = Z_{BH} e^{2\beta i e^{-I_\text{inst eff}}} 
\ee
from which we can read off,
\be 
\Gamma_\text{no backreaction} =  e^{-I_\text{inst eff}} =  Z_{\text{1-loop particle}} e^{- 2\pi Q \left(q - \sqrt{q^2-m^2} \right)}
\ee
which is exactly the result in the literature that neglects backreaction but sums over the contribution of an arbitrary number of instantons.

\subsubsection*{The pair-production including back-reaction: \\ 
black holes with stupendously large charge}

As described in the introduction, black holes that are large have a large instanton action ($I_\text{inst eff.} \gg 1$) regardless of how small the ratio $m/q$ is. This means that we shall take $e^{-I_\text{inst eff.}^k}$ to be the expansion parameter for the pair-production rate. Note that from \eqref{eq:inst-eff-k}, $e^{-I_\text{inst eff.}^k}$ contributes at the same order as $e^{-k I_\text{inst eff.}}$.

Coming back to \eqref{eq:F(u)-exact}, we can now determine the leading order correction from including the effect of having $\alpha \neq 1$. Since we are interested in the effect at small temperatures, one first observable we should understand is whether the presence of defects will affect the spectral edge $E_0$. This amounts to solving $\mathcal F(2 \gamma E_0) = 0$ order by order in $1-\alpha$. 

First, let's neglect the winding solutions. To second order in $1-\alpha$ we find:
\be
\label{eq:E0-shift}
2\gamma E_0 = -2 i e^{-I_\text{inst eff}} + 4\pi^2 e^{-2 I_\text{inst eff}} (1-\alpha)^2 + 16 \pi^4 i e^{-3 I_\text{inst eff}} (1-\alpha)^4 + O\left(e^{-4 I_\text{inst eff}}(1-\alpha)^6\right)
\ee
where each order in $(1-\alpha)$ is exact in terms of $e^{-I_\text{inst eff}}$. Therefore, this should not only be viewed as an expansion in terms of $(1-\alpha)$ but also in  $e^{-I_\text{inst eff}}$. 

Now, including the winding solutions we have 
\be
2 \gamma E_0 &= -2 i \left(\sum_{k=1}^\infty e^{-I_\text{inst eff}^k} \right)+ 4\pi^2 (1-\alpha)^2 \left(\sum_{k=1}^\infty k e^{-I_\text{inst eff}^k} \right)^2 + \nn \\ &+16i \pi^4 (1-\alpha)^4\left(\sum_{k=1}^\infty k e^{-I_\text{inst eff}^k} \right)^2 \left(\sum_{k=1}^\infty k^2 e^{-I_\text{inst eff}^k} \right) + O\left(e^{-4 I_\text{inst eff}}(1-\alpha)^6\right)\,,
\ee
The above expansion should really be understood only as an expansion up to order $O\left(e^{-4 I_\text{inst eff}}\right)$ so not all the exponential terms in the parentheses should be kept.

We should also note that the partition function at low temperatures is given by the density of states around the edge of the spectrum. We shall once again start by neglecting multiple windings. In such a case, expanding \eqref{eq:density-of-states-generating-function} around $E \to E_0$, one finds 
\be 
\rho(E) = \sqrt{2\gamma (E-E_0)}\frac{e^{\pi Q^2}}{2\pi E_{SL(2)}} \underbrace{\int_\mC \frac{dy}{2\pi i} e^{2\pi y} \left(\frac{1}{\sqrt{y^2-2  i e^{-I_\text{inst eff}} e^{-2\pi(1-\alpha)y} - 2 \gamma E_0}}\right)}_{\text{Energy independent const } \equiv\,\, \mC} + O\left(\frac{1}{\sqrt{2\gamma (E-E_0)}}\right)\,,
\ee
where we have defined the energy independent constant $\mC$ which can also be determined in a $1-\alpha$ expansion:
\be
\label{eq:1-loop-further-corr}
\mC = 1 - 4 i \pi^2 e^{-I_\text{inst eff}} (1-\alpha) + 2\pi^2 \left(i e^{-I_\text{inst eff}} - 4 \pi^2 e^{-2I_\text{inst eff}} \right) (1-\alpha)^2 + O\left(e^{-I_\text{inst eff}} (1-\alpha)^3\right)\,.
\ee
Again, including the winding solutions we have 
\be 
\mC &= 1-4\pi^2 i  (1-\alpha)\left(\sum_{k=1}^\infty k\, e^{-I_\text{inst eff}^k} \right) + 2\pi^2 (1-\alpha)^2 \left[\left(\sum_{k=1}^\infty i k^2 \, e^{-I_\text{inst eff}^k} \right) - 4\pi^2 \left(\sum_{k=1}^\infty k \, e^{-I_\text{inst eff}^k}  \right)\right]\nn \\ &+8\pi^4 (1-\alpha)^3\left[3\left(\sum_{k=1}^\infty (-i k) \, e^{-I_\text{inst eff}^k} \right) \left(\sum_{k=1}^\infty (i k^2) \, e^{-I_\text{inst eff}^k} \right) + \frac{4\pi^2}3 \left(\sum_{k=1}^\infty (-ik) \, e^{-I_\text{inst eff}^k}  \right)^3\right] + \nn \\ 
&+ O\left(e^{-2I_\text{inst eff}} (1-\alpha)^4\right)\,.
\ee

The above density of states yields a low temperature partition function given by
\be  
Z_\text{all instantons}(\beta) = \mC \left( \frac{Q^3}{\beta}\right)^{3/2} e^{\pi Q^2 - \beta E_0}\,,
\ee
which thus gives a ratio of partition functions: 
\be  
\frac{Z_\text{all instantons}(\beta)}{Z_\text{BH}(\beta)} = {\mC}  e^{- \beta E_0}\,.
\ee
Finally the fully back-reacted decay rate is given by 
\be 
\Gamma = \frac{1}{\beta} \Im \log\left(\frac{Z_\text{all instantons}(\beta)}{Z_\text{BH}(\beta)}\right) = -\Im E_0 + \Im \frac{1}{\beta} \log {\mC} =_{\beta \to \infty } -\Im E_0 \,,
\ee
which can be easily computed from \eqref{eq:E0-shift} and \eqref{eq:1-loop-further-corr}. Note that at low temperatures the last term can be dropped and we are left with the shift in the spectral edge as the only effect from the instantons.  Consequently, we thus see that neither quantum effects nor gravitational backreaction play a significant role in the pair production rate since further corrections are suppressed in $e^{-I_\text{inst eff}}$. 

Another effect of the quantum backreaction due to the instantons is that we see a small shift of the extremal energy (i.e. the lowest energy  in a sector of fixed charge $Q$) given by 
\be 
2\gamma \Re E_0 =  4\pi^2 e^{-2 I_\text{inst eff}} (1-\alpha)^2  + O\left(e^{-4 I_\text{inst eff}}(1-\alpha)^6\right)\,.
\ee
It is perhaps noteworthy that $\Re E_0>0$ which means that the corrected extremal energy satisfies $E_\text{extremal} = Q+\Re E_0 > Q$. This should however be corrected to further classical corrections that are known to affect the extremality bound such as higher derivative stringy corrections to the extremal energy. 

%%%%%%%%%%%%%%%%%%%%%%%%%%%%%%%%%%%%%%%%%%%%%%%%%%%%%%%%%%%%%%%%%%%%%%%%%
\section{Classical Action for RN}
The classical action for the fixed charge ensemble is
\be
I_{E M}=  -\left[\frac{1}{4}\int d^4 x \sqrt{g}R + \frac{1}{2} \int_{\partial M} \sqrt{h} K\right]+\frac{1}{4} \int d^4 x \sqrt{g} F_{\mu \nu} F^{\mu \nu}- \int_{\partial M} \sqrt{h} n_i F^{i j} A_j ,
\ee
\be
A = i Q \lrm{\frac{1}{r}-\frac{1}{r_+}} dt, \qquad F = \frac{i Q}{r^2} dt \wedge d r, \qquad F^2 = -\frac{2 Q^2}{r^4}\,. 
\ee
\be
K =  \frac{d \log [\textrm{area}]}{ds} =  \frac{\partial r}{\partial s}  \frac{\partial_r ( \chi r^2)} { \chi r^2} = \chi   \frac{\partial_r ( \chi^2 r^4)} { 2\chi^2 r^4}  = \frac{1}{\chi} \left( \frac{M}{r^2} - \frac{Q^2}{r^3}  \right)  + \frac{2 \chi}{r}  \ . 
\ee
With $K_0 = \frac{2}{r}$ as $r \to \infty$. The individual contributions are
\be
I_{\t{bdy}} = -\frac{1}{2} \times 4 \pi \int d \tau \lim_{r \to \infty} r^2 (K-K_0) = 2 \pi \beta M\,.
\ee
\be
I_{F^2 \t{ bulk}} = \frac{1}{4} 4 \pi \beta \int_{r_+}^\infty d r r^2 \frac{-2 Q^2}{r^4} = -\frac{2\pi Q^2 \beta}{r_+}\,.
\ee
\be
I_{F^2 \t{ bdy}} = (-1)^2 4 \pi \beta \lim_{r \to \infty} r^2 \frac{Q^2}{r^2} (\frac{1}{r}-\frac{1}{r_+})  = \frac{4\pi Q^2 \beta}{r_+} + \t{counter-term}\,.
\ee
There are two actions we can compute, with and withouth the EM boundary term. In \MU{[Gibbons/Hawking]} they do the computation without the boundary term and find the answer
\be
I_{\t{Gibbons/hawking}} = \beta (M - \frac{Q^2}{r_+})\.
\ee
Our answer is given by
\be
I_{\t{bdy}}+I_{F^2 \t{ bulk}} = 2 \pi \beta (M - \frac{Q^2}{r_+})\,.
\ee
Which is consistent with what they found. However, to calculate the partition function at fixed charge we need the boundary term which gives 
\be
I_{EM}=2 \pi \beta (M + \frac{Q^2}{r_+}) = -4 \pi (\pi Q^2 - \beta Q + 2\pi^2 Q^3 T + \ldots)\,
\ee
Which is the expected answer.
